# Supplementary material for: On the Alignment of Group Fairness with Attribute Privacy
Source: arXiv:2211.10209 source file (2024-03-05)
Supplement: Supplementary file 1 [file 10appendix.tex]

\appendix

\section*{Appendix}

We detail here more details about the notations, and proofs supporting the theorems presented in the paper.

\section{Notations}
%\section{More Details on the Notations}
\label{app:notations}

We introduce some notations from probability theory to formalize ML which will be used in the rest of the paper. Let $A$ be a set.
The set of subsets of $A$ is $\mathcal{P}(A)$. 
Each element $a \in \mathcal{P}(A)$ is such that $a \subset A$.
A tribe $\mathcal{A}$ is a subset of $\mathcal{P}(A)$ that contains $\emptyset$, $A$ and is stable by complementary and countable union.
We say that $(A,\mathcal{A})$ is a measurable space.
A measure $d$ is a function $d$:$\mathcal{A}$ $\rightarrow$ $[0,+\infty]$ such that $d(\emptyset) = 0$ and $d\left(\bigcup_{i\in \mathbb{N}} A_i\right) = \sum_{i\in \mathbb{N}}d(A_i)$ for any $(A_1, A_2, \cdots) \in \mathcal{A}^\mathbb{N} $ with $\forall (i,j) A_i\cap A_j = \emptyset$.
We then say that $(A, \mathcal{A}, d)$ is a measure space.
Any function mapping $A$ to $B$ is called a measurable function if $\forall b\in\mathcal{B}$~$f^{-1}(b)\in\mathcal{A}$ and we note $f:(A, \mathcal{A})\rightarrow (B, \mathcal{B})$ or $f:(A, \mathcal{A},d)\rightarrow (B, \mathcal{B})$

In the special case where $d(A) = 1$ we call $d$ a probability measure.
We then call $(A,\mathcal{A},d)$ a probability space and the measurable functions on this space are called random variables.

$\hat{S} = 1_{[0.5,1]}\circ a\circ f_{target}\circ X$ translates to $S$ is equal to the composition of four functions: the random variable $X$, the target model $f_target$, the attack model $a$ and the indicator function of the set [0.5,1].

\begin{table}[!htb]
\caption{Summary of notations used in the paper.}
\begin{center}
\begin{tabular}{ | c | c | }
\hline
\textbf{Notation} & \textbf{Meaning}\\
\hline
 \adv & Adversary \\  
 $\targetmodel$ & Target model being attacked \\
 $\targetmodel\circ X$ & \\
 $ \hat{Y}=1_{[\tau,1]}\circ \targetmodel\circ X$ & \\
 $\attackmodel$ & Attack model used by adversary \\  
 $\traindata$ & Data used to train the target model \\  
 $\testdata$ & Data used to test the target model \\  
 $\auxdata$ & Auxiliary data available to the adversary \\
 $\auxtraindata$ & Adversary's dataset to train attack model\\
 $\auxtestdata$ & Adversary's dataset to evaluate attack model\\
 $X$ & \\
 $Y$ & \\
 $S$ & \\
 $X(\omega), Y(\omega), S(\omega)$ & Specific instances parameterized by $\omega$\\
 $(\Omega, \mathcal{T}, \mathcal{P})$ & \\
 $E, \mathcal{U}$ & \\
$\mathcal{B}$ & \\
 \hline
\end{tabular}
\end{center}
\label{tab:notations}
\end{table}

\section{Balanced AIA accuracy under DP fairness constraints}
\label{app:dp}

\begin{proof}
We have seen in section \ref{sec:atthard} that the set $B$ of function from $\{0,1\}$ to $\{0,1\}$ contains four elements $b_0$, $b_1$, $b_2$ and $b,3$.
For every $b\in B$ the balanced \aia accuracy is 
$BA(b) = \frac{1}{2}(P(b\circ \hat{Y}=0|S=0) + P(b\circ \hat{Y}=1|S=1))$.
We have $BA(b_0) = BA(b_3) = \frac{1}{2}$ hence we can discard those elements when solving the attack optimisation problem.
This problem writes $\text{max}_{b\in B}B(A(b)) = \text{max}(BA(b_1), BA(b_2))$.
We remark that $b_1\circ \hat{Y}=\hat{Y}$ and $b_2\circ \hat{Y}=1 - \hat{Y}$.
Hence,
{\footnotesize
\begin{align*}
    BA(b_1) &= \frac{1}{2}(P(\hat{Y}=0|S=0) + P(\hat{Y}=1|S=1))\\
    &=\frac{1}{2}(1+P(\hat{Y}=1|S=1) - P(\hat{Y}=1|S=0))
\end{align*}
}
And
{\footnotesize
\begin{align*}
    BA(b_2)=\frac{1}{2}(1+P(\hat{Y}=1|S=0) - P(\hat{Y}=1|S=1))
\end{align*}
}
Thus,
{\footnotesize
\begin{align*}
    &\text{max}_{b\in B}BA(b) \\
    = &\frac{1}{2}\left(1+\text{max}\left(
    \begin{matrix}
        P(\hat{Y}=0|S=0) -P(\hat{Y}=1|S=1)\\ 
        P(\hat{Y}=1|S=0) -P(\hat{Y}=0|S=1)
    \end{matrix}
    \right)\right)\\
    =&\frac{1}{2}(1+|P(\hat{Y}=1|S=1) - P(\hat{Y}=1|S=0)|)
\end{align*}
}
%Let $\hat{Y}:\Omega\rightarrow\{0,1\}$ be a random variable that satisfies \demparity for $S$ and $\hat{S}$ be the inferred sensitive attribute from the attack classifier on exploiting $\hat{Y}$. Then,
%\begin{equation}
%\label{eq:defShat}
%    \hat{S}=1_{[\upsilon,1]}\circ \attackmodel\circ \hat{Y},
%\end{equation}
%where $\upsilon\in[0,1]$ and $\attackmodel:\{0,1\}\rightarrow[0,1]$ is a measurable function.

%We compute the balanced \aia accuracy to infer $\hat{S}$, given by, $\frac{1}{2}(P(\hat{S}=1|S=1)+P(\hat{S}=0|S=0))$.
%In this expression, we substitute the definition of $\hat{S}$ from Equation~\ref{eq:defShat} which gives us the conditional law of $Y$ knowing $S$.
%Using the Definition~\ref{def:dp}, we can compute the balanced \aia accuracy when training with \demparity.
%{
%\footnotesize
%\begin{align*}
%    &\frac{1}{2}(P(\hat{S}=1|S=1)+P(\hat{S}=0|S=0))\\
%    =&\frac{1}{2}(P({1_{[\upsilon,1]}\circ \attackmodel\circ\hat{Y}=1|S=1}) + %P({1_{[0,\upsilon]}\circ \attackmodel\circ\hat{Y}=0|S=0}))\\
%    =&\frac{1}{2}(P({\hat{Y}\in \attackmodel^{-1}([\upsilon,1])|S=1}) + P({\hat{Y}\in %\attackmodel^{-1}([0,\upsilon])|S=0})\\
%    =&\frac{1}{2}(1-P({\hat{Y}\in \attackmodel^{-1}([0,\upsilon])|S=1})+P({\hat{Y}\in %\attackmodel^{-1}([0,\upsilon])|S=0})\\
%    =&\frac{1}{2}(1-P({\hat{Y}\in \attackmodel^{-1}([0,\upsilon])|S=0})+P({\hat{Y}\in %\attackmodel^{-1}([0,\upsilon])|S=0})\\
%    =&\frac{1}{2}
%\end{align*}
%}
\end{proof}

\section{Balanced AIA accuracy under EO fairness constraints}
\label{app:eo}

\begin{proof}
    Let $\hat{Y}:\Omega\rightarrow\{0,1\}$ a random variables classifier of $Y$ that satisfies \eo for $S$.
    Let $\hat{S}$ an attack classifier of $S$ using $\hat{Y}$ with the same definition as in equation \ref{eq:defShat}.
    For this proof, we use the total probability law to make use of the conditional law of $\hat{Y}$ knowing $(S,Y)$.
    {
    \footnotesize
    \begin{align}
         &\frac{1}{2}(P(\hat{S}=1|S=1)+P(\hat{S}=0|S=0))\\
        =&\frac{1}{2}(P({1_{[\upsilon,1]}\circ \attackmodel\circ\hat{Y}=1|S=1}) + P({1_{[0,\upsilon}]\circ \attackmodel\circ\hat{Y}=0|S=0}))\\
        =&\frac{1}{2}(P({\hat{Y}\in \attackmodel^{-1}([\upsilon,1])|S=1}) + P({\hat{Y}\in \attackmodel^{-1}([0,\upsilon])|S=0})\\
        =&\frac{1}{2}(1-P({\hat{Y}\in \attackmodel^{-1}([0,\upsilon])|S=1})+P({\hat{Y}\in \attackmodel^{-1}([0,\upsilon])|S=0})
        \label{eq:expbaeo}
    \end{align}
    }
    Then we use the total probability law for $P({\hat{Y}\in \attackmodel^{-1}([0,\upsilon])|S=1})$ and $P({\hat{Y}\in \attackmodel^{-1}([0,\upsilon])|S=0})$
    {
    \footnotesize
    \begin{align*}
        &P({\hat{Y}\in \attackmodel^{-1}([0,\upsilon])|S=1})\\
        =&P({\hat{Y}\in \attackmodel^{-1}([0,\upsilon])|S=1,Y=1})P(Y=1|S=1)+\\
        &P({\hat{Y}\in \attackmodel^{-1}([0,\upsilon])|S=1,Y=0})P(Y=0|S=1)
    \end{align*}
    }
    {
    \footnotesize
    \begin{align*}
        &P({\hat{Y}\in \attackmodel^{-1}([0,\upsilon])|S=0})\\
        =&P({\hat{Y}\in \attackmodel^{-1}([0,\upsilon])|S=0,Y=1})P(Y=1|S=0)+\\
        &P({\hat{Y}\in \attackmodel^{-1}([0,\upsilon])|S=0,Y=0})P(Y=0|S=0)\\
    \end{align*}
    }
     Because $\hat{Y}$ satisfies \eo we have 
    \begin{align*}
        &P({\hat{Y}\in \attackmodel^{-1}([0,\upsilon])|S=1,Y=1})P(Y=1|S=1)+\\
        &P({\hat{Y}\in \attackmodel^{-1}([0,\upsilon])|S=1,Y=0})P(Y=0|S=1)\\
        =&P({\hat{Y}\in \attackmodel^{-1}([0,\upsilon])|S=0,Y=1})P(Y=1|S=1)+\\
        &P({\hat{Y}\in \attackmodel^{-1}([0,\upsilon])|S=0,Y=0})P(Y=0|S=1)\\
    \end{align*}
    
    Finally we substitute $P({\hat{Y}\in \attackmodel^{-1}([0,\upsilon])|S=1})$ and \\$P({\hat{Y}\in \attackmodel^{-1}([0,\upsilon])|S=0})$ in equation 
    \ref{eq:expbaeo}.
    {
    \footnotesize
    \begin{align*}
        &\frac{1}{2}(P(\hat{S}=1|S=1)+P(\hat{S}=0|S=0))=\\
        &\frac{1}{2}
        P({\hat{Y}\in \attackmodel^{-1}([0,\upsilon])|S=0,Y=0})(P(Y=0|S=0) - P(Y=0|S=1))+\\
        &\frac{1}{2}P({\hat{Y}\in \attackmodel^{-1}([0,\upsilon])|S=0,Y=1})(P(Y=1|S=0) - P(Y=1|S=1))+\\
        &\frac{1}{2} = \\
        &\frac{1}{2}
        P({\hat{Y}\in \attackmodel^{-1}([0,\upsilon])|S=0,Y=0})(P(Y=0|S=0) - P(Y=0|S=1))+\\
        &\frac{1}{2}P({\hat{Y}\in \attackmodel^{-1}([0,\upsilon])|S=0,Y=1})(-P(Y=0|S=0) + P(Y=0|S=1))+\\
        &\frac{1}{2} = \\
        &\frac{1}{2}(P(Y=0|S=0) - P(Y=0|S=1))\\
        &\left(P({\hat{Y}\in \attackmodel^{-1}([0,\upsilon])|S=0,Y=0}) - P(\hat{Y}\in \attackmodel^{-1}([0,\upsilon])|S=0,Y=1)\right) +\\
        &\frac{1}{2}
    \end{align*}
    }
In conclusion, the balanced accuracy of $\hat{S}$ is equal to $\frac{1}{2}$ if and only if $P(Y=0|S=0) = P(Y=0|S=1)$ or $P({\hat{Y}\in \attackmodel^{-1}([0,\upsilon])|S=0,Y=0}) = P(\hat{Y}\in \attackmodel^{-1}([0,\upsilon])|S=0,Y=1)$. So either $S$ is independent of $Y$ or $\hat{Y}$ is independent of $Y$.
\end{proof}

\section{No Guarantee of Differential Privacy}
\label{app:dp}

While Differential Privacy (DP) aims to make the participation of individuals indistinguishable to an observer accessing the results of a computation, fairness attempts to equalize the properties of those results between different individuals. 
Here we prove that DP does not give any guarantee of protection against sensitive attribute inference attacks. To do this we consider a DP training mechanism with $\epsilon=0$ (i.e., an upper bound of the protection) as well as an attack model where XXX never cheat (i.e., 100\% accuracy).

Let ($\rho$, A, P) be a probability space. Let also (F(E, F), B) be a space
measurable. E is the Cartesian product of n sets, the s-th being the sensitive attribute. E represents the n features. F = Es.
We give ourselves the random mechanism

$$formula ,$$
where F(E, F) est l’ensemble des fonctions de E dans F, and  V A(A, B) est l’ensemble de variables al´eatoires de A dans B

$$formula$$

M therefore satisfies the differential confidentiality for = 0. This is the strongest guarantee of differential confidentiality possible. And yet sensible attribute inference from hard labels works perfectly using identity as an attack model. By “works perfectly” we mean that the model is never wrong: it has an accuracy of 100\%.

\section{Evaluation setup: dataset splits}
\label{app:dataset}

\begin{table}[!htb]
\footnotesize
\begin{center}
\caption{Summary of dataset splits.}
\begin{tabular}{ | c | c | c | c | c |}
\hline
\rowcolor{LightCyan}  \textbf{Dataset} & |$\traindata$| & |$\testdata$| & |$\auxtraindata$| & |$\auxtestdata$|\\ 
\hline
 \textbf{\census} & 24,752 & 6,188 & 4,950 & 1,238\\  
 \textbf{\compas} & 4,937 & 1,235 &988 & 247\\  
\textbf{\meps} & 12,664 & 3,166 & 2,532 & 634\\  
 \textbf{\law} & 16,368 & 4,092 & 3,273 & 819\\  
\textbf{\credit} & 24,000 & 6,000 & 4,800 & 1,200\\  
  \hline
\end{tabular}
\end{center}
\label{tab:dataset}
\end{table}
